# Supplementary material for: EQ-VAE: Equivariance Regularized Latent Space for Improved Generative Image Modeling
Source: arXiv:2502.09509 source file (2025-08-04)
Supplement: Supplementary file 1 [file fig_appendix_gen.tex]

{
\small
\centering
\newcommand{\resultsfignew}[1]{\includegraphics[width=0.12\textwidth,valign=c]{#1}}
\setlength{\tabcolsep}{1pt}

\begin{tabular}{@{}cccccc@{}}
    
    \mc{6}{Class label = “panda” (388)} \\

    \resultsfignew{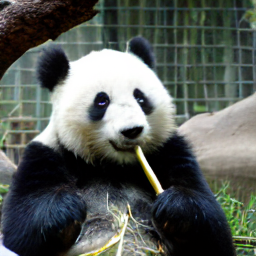} & 
    \resultsfignew{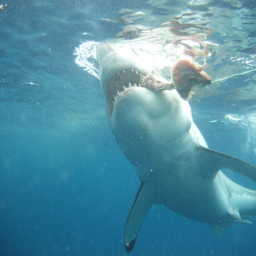} & 
    \resultsfignew{fig/latent_latex/im-1.png} &     \resultsfignew{fig/latent_latex/im-1.png} & 
    \resultsfignew{fig/latent_latex/im-1.png} & 
    \resultsfignew{fig/latent_latex/im-1.png}  \\

    \mc{6}{\vspace{-2.0ex}}\\

    \resultsfignew{fig/latent_latex/im-1.png} & 
    \resultsfignew{fig/latent_latex/im-1.png} & 
    \resultsfignew{fig/latent_latex/im-1.png} &     \resultsfignew{fig/latent_latex/im-1.png} & 
    \resultsfignew{fig/latent_latex/im-1.png} & 
    \resultsfignew{fig/latent_latex/im-1.png}  \\
    
    \mc{6}{\vspace{-2.0ex}}\\

    \resultsfignew{fig/latent_latex/im-1.png} & 
    \resultsfignew{fig/latent_latex/im-1.png} & 
    \resultsfignew{fig/latent_latex/im-1.png} &     \resultsfignew{fig/latent_latex/im-1.png} & 
    \resultsfignew{fig/latent_latex/im-1.png} & 
    \resultsfignew{fig/latent_latex/im-1.png}  \\

    \mc{6}{\vspace{-1.ex}}\\
    
    \mc{6}{Class label = “lion” (291)
} \\

    \resultsfignew{fig/latent_latex/im-1.png} & 
    \resultsfignew{fig/latent_latex/im-1.png} & 
    \resultsfignew{fig/latent_latex/im-1.png} &     \resultsfignew{fig/latent_latex/im-1.png} & 
    \resultsfignew{fig/latent_latex/im-1.png} & 
    \resultsfignew{fig/latent_latex/im-1.png}  \\

    \mc{6}{\vspace{-2.0ex}}\\

    \resultsfignew{fig/latent_latex/im-1.png} & 
    \resultsfignew{fig/latent_latex/im-1.png} & 
    \resultsfignew{fig/latent_latex/im-1.png} &     \resultsfignew{fig/latent_latex/im-1.png} & 
    \resultsfignew{fig/latent_latex/im-1.png} & 
    \resultsfignew{fig/latent_latex/im-1.png}  \\

    \mc{6}{\vspace{-2.0ex}}\\

    \resultsfignew{fig/latent_latex/im-1.png} & 
    \resultsfignew{fig/latent_latex/im-1.png} & 
    \resultsfignew{fig/latent_latex/im-1.png} &     \resultsfignew{fig/latent_latex/im-1.png} & 
    \resultsfignew{fig/latent_latex/im-1.png} & 
    \resultsfignew{fig/latent_latex/im-1.png}  \\

    \mc{6}{\vspace{-1.ex}}\\

    \mc{6}{Class label = “balloon” (417)} \\

    \resultsfignew{fig/latent_latex/im-1.png} & 
    \resultsfignew{fig/latent_latex/im-1.png} & 
    \resultsfignew{fig/latent_latex/im-1.png} &     \resultsfignew{fig/latent_latex/im-1.png} & 
    \resultsfignew{fig/latent_latex/im-1.png} & 
    \resultsfignew{fig/latent_latex/im-1.png}  \\

    \mc{6}{\vspace{-2.0ex}}\\

    \resultsfignew{fig/latent_latex/im-1.png} & 
    \resultsfignew{fig/latent_latex/im-1.png} & 
    \resultsfignew{fig/latent_latex/im-1.png} &     \resultsfignew{fig/latent_latex/im-1.png} & 
    \resultsfignew{fig/latent_latex/im-1.png} & 
    \resultsfignew{fig/latent_latex/im-1.png}  \\

    \mc{6}{\vspace{-2.0ex}}\\

    \resultsfignew{fig/latent_latex/im-1.png} & 
    \resultsfignew{fig/latent_latex/im-1.png} & 
    \resultsfignew{fig/latent_latex/im-1.png} &     \resultsfignew{fig/latent_latex/im-1.png} & 
    \resultsfignew{fig/latent_latex/im-1.png} & 
    \resultsfignew{fig/latent_latex/im-1.png}  \\
    
\end{tabular}
}
