# Supplementary material for: EQ-VAE: Equivariance Regularized Latent Space for Improved Generative Image Modeling
Source: arXiv:2502.09509 source file (2025-08-04)
Supplement: Supplementary file 2 [file tab_autoencoders_comp_appendix.tex]

\begin{table}[t]
%\footnotesize
\label{tab:comp_auto}
\centering
\setlength{\tabcolsep}{2.3pt} % Adjust column spacing
\scalebox{0.78}{
\begin{tabular}{cccccccc}
\toprule
& \multirow{2}{*}{\Th{Autoencoder}}  & \mc{4}{Reconstruction} & \mc{2}{Generation} \\ 
\cmidrule(lr){3-6} \cmidrule(lr){7-8}
& & \Th{rFID$\downarrow$} & \Th{PSNR $\uparrow$} & \Th{LPIPS $\downarrow$} &  \Th{SSIM $\uparrow$} & \Th{gFID$\downarrow$} & \Th{IS$\uparrow$}\\ 
\midrule 
 & \sdvae  & $0.90$ & $25.82$ & $0.146$ & $0.71$ & $43.5$ & $?$\\
 & \textbf{w/ \our (ours)}   & $0.82$& $25.95$ & $0.141$ & $0.72$ & $34.1$ & $?$\\ \addlinespace
\cline{2-8}
\addlinespace
\vspace{-10.0pt}
\multirow{6}{*}{\rotatebox{90}{\Th{Cont.}}} & & & & & &\\

 & \sdxlvae  & $0.67$ & $27.36$ & $0.121$ & $0.76$ & $46.0$ & $?$\\
 & \textbf{w/ \our (ours)}  & $0.65$ & $27.48$ & $0.118$ & $0.76$  & $35.9$ & $?$\\ \addlinespace
\cline{2-8}
 \addlinespace

 & \texttt{SD3-VAE}  &  $0.20$  & $31.27$ & $0.060$ & $0.87$ & $58.9$ & $?$\\
 & \textbf{w/ \our (ours)} &  $0.19$  & $31.06$ & $0.061$ & $0.87$ & $54.0$ & $?$\\ 

\addlinespace
\cline{2-8}
 \addlinespace

 & \texttt{SD-VAE-16}  &  $0.87$  & $24.67$ & $0.161$ & $0.61$ & $80.2$ & $?$\\
 & \textbf{w/ \our (ours)} &  $0.82$  & $25.21$ & $0.152$ & $0.69$ & $64.1$ & $?$\\ 

 \bottomrule
 
 \addlinespace

\multirow{2}{*}{\rotatebox{90}{\Th{Disc.}}} & \texttt{VQ-GAN} & $?$ & $?$ & $?$ & $?$ & $?$ & $?$\\
 & \textbf{w/ \our (ours)} & $?$  & $?$& $?$ & $?$ & $?$ & $?$\\ \addlinespace
\bottomrule
\end{tabular}
}
\vspace{-3pt}
\caption{\textbf{Performance enhancement on different autoencoders}. gFID on \texttt{DiT-B/2}}
\label{tab:bench-diff}
\vspace{-3pt}
\end{table}
